# Supplementary material for: Implicit Rate-Constrained Optimization of Non-decomposable Objectives
Source: arXiv:2107.10960 source file (2021-07-29)
Supplement: Supplementary file 1 [file appendix.tex]

\section{Additional Experiments}
\label{app:expts}

\begin{figure*}
    \centering
    \begin{subfigure}{0.33\textwidth}
    \centering
    \includegraphics[width=0.99\columnwidth]{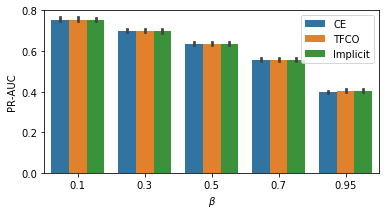}
    \caption{Adult}
    \end{subfigure}
    \begin{subfigure}{0.33\textwidth}
    \centering
    \includegraphics[width=0.99\columnwidth]{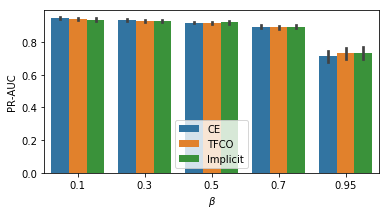}
    \caption{Spambase}
    \end{subfigure}
    \begin{subfigure}{0.33\textwidth}
    \centering
    \includegraphics[width=0.99\columnwidth]{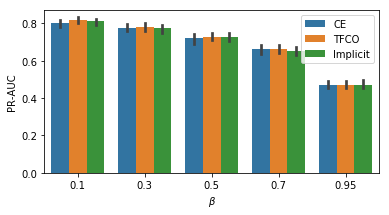}
    \caption{Crime}
    \end{subfigure}
    \caption{Plot of PR-AUC in $[\beta, 1]$ as a function of $\beta$.} %
    \label{fig:prauc-app}
\end{figure*}
